# Supplementary material for: Modeling Psychotherapy Dialogues with Kernelized Hashcode Representations: A Nonparametric Information-Theoretic Approach
Source: arXiv:1804.10188 source file (2019-09-09)
Supplement: Supplementary file 1 [file appendix.tex]

\appendix

\section{Derivations of the Information Theoretic Bounds
% LB and Entropy UB
% Derivation
}
\label{sec:bounds_deriv}
% \vspace{-2mm}
% 
Before the discussion of our novel lower bound of mutual information, we introduce the information-theoretic quantity called \textit{Total Correlation}~($\mathcal{TC}$), which captures non-linear correlation among the dimensions of a random variable $\bs{C}$, i.e., 
% 
% \vspace{-2mm}
\begin{align}
&
\cT\cC(\bs{C}) = \sum\limits_j \cH(C_j) - \cH(\bs{C});
\vspace{-4mm}
\end{align}
For a 2-D random variable, total correlation corresponds to mutual information quantity itself. 
And, $\cT\cC(\bs{C}: \bs{Y})$ is defined as,
\vspace{-3mm}
\begin{align}
\nonumber
\\
&
\cT\cC(\bs{C}: \bs{Y}) = \cT\cC(\bs{C}) - \cT\cC(\bs{C}|\bs{Y}).
\label{eqn:corex}
% \vspace{-4mm}
\end{align}
Intuitively, \eqnref{eqn:corex} describes the amount of information within $\bs{C}$ that can be explained by $\bs{Y}$.
% 
% The interesting aspect of this quantity $\cT\cC(\bs{\cX}: \bs{\cY}; M_h)$ is that one can compute $\cT\cC(\bs{\cX}: \bs{\cY}; M_h)$ efficiently for $\bs{\cY}$ is such that it maximizes the quantity, i.e., when $\bs{\cY}$ explains all the correlations present in $\bs{\cX}$. In this scenario, $p(\bs{x}|\bs{y}; M_h)$ factorizes, as per the \emph{Naive Bayes} model $p(\bs{x}|\bs{y}; M_h)=\prod_{j}p(\bs{x}(j)|\bs{y}; M_h)$, thus making the computations cheap~\cite{greg2014discovering}. 

Along these lines, the mutual information quantity between the hashcodes can be decomposed as in \lmaref{lma:mi_decompose} below.
% 	
% \vspace{-1mm}
\begin{lemma}[Mutual Information Decomposition]
\label{lma:mi_decompose}
Mutual Information between $\bs{C^t}$ and $\bs{C^p}$ is decomposed as follows:
% 
% \vspace{-3mm}
\begin{align}
&
\cI(\bs{C^t}: \bs{C^p})
% \nonumber
% \\
% &
% = \cH(\bs{\cC_t}; M_h) - \cH(\bs{\cC_t} | \bs{\cC_p}; M_h)
% 
% \nonumber\\
% &= \sum\limits_i {\cH(\bs{\cC_t}(i))}-\sum\limits_i {\cH(\bs{\cC_t}(i) | \bs{\cC_p})} \nonumber \\
% &~~~~
% + \cH(\bs{\cC_t}) - \cH(\bs{\cC_t} | \bs{\cC_p}) \nonumber \\
% &~~~~
% - \sum\limits_i {\cH(\bs{\cC_t}(i))}
% +
% \sum\limits_i {\cH(\bs{\cC_t}(i) | \bs{\cC_p})} \nonumber \\
% &
% = \sum\limits_i {\cI(\bs{\cC_t}(i): \bs{\cC_p})} - (\cT\cC(\bs{\cC_t}) - \cT\cC(\bs{\cC_t}|\bs{\cC_p})) 
\nonumber 
\\
&
= \sum\limits_j {\cI(C^t_j: \bs{C^p})} -
\cT\cC(
\bs{C^t}: \bs{C^p}).
\label{eqn:deco_mi}
% \vspace{-3mm}
\end{align}
% \vspace{-4.5mm}
\begin{proof}
\begin{align*}
\cI(\bs{C^t}: \bs{C^p})
&
= \cH(\bs{C^t}) - \cH(\bs{C^t} | \bs{C^p})
\nonumber \\
&
= 
\sum\limits_j
\cH(C^t_j) 
- 
\sum\limits_j
\cH(C^t_j | \bs{C^p})
+ \cH(\bs{C^t}) 
\nonumber \\
&
- \cH(\bs{C^t} | \bs{C^p})
- \sum\limits_j {\cH(C^t_j)}
+
\sum\limits_i {\cH(C^t_i | \bs{C^p})} \nonumber \\
&
= \sum\limits_j {\cI(C^t_j: \bs{C^p})} - (\cT\cC(\bs{C^t}) - \cT\cC(\bs{C^t}|\bs{C^p}))
\nonumber 
\\
&
= \sum\limits_j {\cI(C^t_j: \bs{C^p})} -
\cT\cC(
\bs{C^t}: \bs{C^p}).
\end{align*}
\end{proof}
\end{lemma}
% 	
% \noindent wherein $\bs{\cC_t}(j)$ denotes the $j_{th}$ dimension of $\bs{\cC_t}$ in \eqnref{eqn:deco_mi}.
% 		
Looking at the first term of RHS in \eqnref{eqn:deco_mi}, it is the mutual information between a one-dimensional and multi-dimensional random variable. 

For these terms, since one of the variables is only 1-D, we can use the existing technique of variational bounds for an approximation, as in \lmaref{lma:variational_lb_mi} below.
% 					
% \vspace{-1.0mm}
\begin{lemma}
\label{lma:variational_lb_mi}
Marginal mutual information for each bit in therapist hashcodes, $\cI(C^t_j: \bs{C^p})$, is lower bounded as,
% 
% \vspace{-3mm}
\begin{align}
% &
\cI(C^t_j: \bs{C^p}) 
\ge 
% \nonumber
% \\
% &
\cH(C^t_j)
+
\left\langle \log q(C^t_j|\bs{C^p})
\right\rangle_{p(C^t_j,\bs{C^p})}.
\label{eqn:vmi}
% \vspace{-3mm}
\end{align}
% 
% \todo{mention, we simply use a variational upper bound on the marginal conditional entropy term. Mention the bound gap.}
% 
\label{lma:marginal_mi_lb}
% \vspace{-5.5mm}
\end{lemma}
\noindent Herein, $\cH(C^t_j)$ is easy to compute because $C^t_j$ is a one-dimensional binary variable. For each of the proposal distributions $q(C^t_j|\bs{C_p})$, we propose to use a Random Forest~(RF) classifier~\cite{gao2016variational}.
            		
In reference to the second term of RHS in \eqnref{eqn:deco_mi}, 
% as mentioned above, 
it is computationally intractable to compute the total correlation expression $\cT\cC(\bs{C^t}:\bs{C^p})$, which denotes the total correlations between bits of $\bs{C^t}$, explainable by $\bs{C^p}$. So, we would also like to obtain an upper bound of $\cT\cC(\bs{C^t}:\bs{C^p})$, which is cheap to compute, that would give us a lower bound for the second term in \eqnref{eqn:deco_mi} because of the negative sign.
\begin{lemma}
$\cT\cC(\bs{C^t}:\bs{C^p})$ is upper bounded as: 
% \vspace{-2mm}
\begin{align}
\cT\cC(\bs{C^t}:\bs{C^p})
\leq
\cT\cC(\bs{C^t}:\bs{Y^*})
\label{eqn:corex_lb}
% \vspace{-4mm}
\end{align}
% 	
% \begin{align}
% \bs{\cY^*}
% \gets
% \mathop{\arg\max}
% \limits_{\bs{\cY}:|\bs{\cY}|=|\bs{\cC_p}|} \cT\cC(\bs{\cC_t}:\bs{\cY}; M_h),
% \label{eqn:corex_opt}
% \end{align}
% 	
% To obtain the upper bound, we aim to solve the optimization problem in \eqnref{eqn:corex_opt} and obtain,
% 	
% 				
\noindent wherein $|.|$ denotes the dimensionality of a random variable.
% in \eqnref{eqn:corex_lb}. 
\label{lma:tc_ub}
% \vspace{-4mm}
\end{lemma}
% 		
% As mentioned previously, 
Although it is intractable to compute the original term $\cT\cC(\bs{C^t}:\bs{C^p})$, it is possible to compute $\cT\cC(\bs{C^t}:\bs{Y^*})$ for a latent variable representation $\bs{Y^*}$ of $\bs{C^t}$ that maximally explains the Total Correlations in $\bs{C^t}$.
% ~\eqnref{eqn:corex_opt}.

% 	
% We discuss more details on obtaining such latent representation in the following.
% 
% 	
We can think of the computation of the upper bound as an unsupervised learning problem. We propose to use an existing algorithm, \emph{CorEx}, for the unsupervised learning of latent random variables representation $\bs{Y^*}$~\cite{greg2014discovering}.
	
% \begin{align}
% \cI(\bs{\cC_t}: \bs{\cC_p}) \ge \sum\limits_i{\cH(\bs{\cC_t}(i)) + \left\langle \log q(\bs{\cC_t}(i)|\bs{\cC_p})\right\rangle_{p(\bs{\cC_t}(i),\bs{\cC_p})}} 
% \\
% - \mathop{\max }\limits_{|\bs{\cY}|=|\bs{\cC_p}|} \cT\cC(\bs{\cC_t};\bs{\cY})
% \label{eqn:mi_lb}
% \end{align}

% We can view the last term of RHS in Eq.~\ref{eqn:mi_lb} 
		
It is important to note some practical considerations about the upper bound. In the case of a suboptimal solution to the maximization of $\cT\cC(\bs{C^t}:\bs{Y})$ above, the optimized quantity may not be an upper bound of $\cT\cC(\bs{C^t}:\bs{C^p})$, but rather an approximation. Also, the upper bound would not be tight if $\bs{C^p}$ doesn't explain much of total correlations in $\bs{C^t}$. Further, for even more computation cost reductions during the learning, the dimension of the latent representation $\bs{Y}$ can be kept much smaller than the dimension of hashcodes, i.e. $|\bs{Y}| \ll |\bs{C^p}|$ for $|\bs{C^p}| \gg 1$; this is because even a small number of latent variables should explain most of the total correlations for practical purposes as demonstrated by \cite{greg2014discovering}, and observed in our experiments on hashcodes as well.
		
% \todo{we can keep size of $\cY$ small as many of the remaining latent variables would contribute very low value.}
	
Combining \eqnref{eqn:vmi} and \eqnref{eqn:corex_lb} into \eqnref{eqn:deco_mi}, we get the lower bound in \thmref{thm:mi_lb}.

Along same lines, we can derive the tight upper bound on joint entropy of hashcodes so as to obtain the normalization of the MI LB.
From the definition of Total Correlation above~\eqnref{eqn:corex}, we have the following,
% 
% \vspace{-2.5mm}
\begin{align*}
&
\sum\limits_j{\cH(C^t_j)}
-
\cT\cC(\bs{C^t})
=
\cH(\bs{C^t}),
\\
&
\cT\cC(\bs{C^t})
=
\cT\cC(\bs{C^t}:\bs{Y^*})
+
\cT\cC(\bs{C^t}|\bs{Y^*}),
% \vspace{-4mm}
\end{align*}
and finally the expression below.
% 
% \vspace{-3mm}
\begin{align*}
&
\sum\limits_j{\cH(C^t_j)}
-
\cT\cC(\bs{C^t}:\bs{Y^*})
\\
&=
\cH(\bs{C^t})
+
\cT\cC(\bs{C^t}|\bs{Y^*})
% \vspace{-3mm}
\end{align*}
From this derived expression, we can simply obtain the upper bound and the corresponding gap.
        
\textbf{Previous Lower Bounds for Mutual Information: 
% outside Dialog Modeling Settings
}
Variational lower bounds on the mutual information criterion have been proposed in the past ~\cite{barber2003algorithm,chalk2016relevant,gao2016variational,chen2016infogan,alemi2017deep,garg2018efficient}.
Their lower bounds works only when one of the variables is fixed, say if $\bs{C^t}$ were fixed. In our objective, not only $\bs{C^t}$ is a functional of the hashing model that we are learning, it is high dimensional. Unless we have a lower bound for the entropy term $\cH(\bs{C^t})$ as well, which should be hard to obtain, we can not use the above mentioned variational lower bounds for our problem as such.
% 
% However, if we apply the variational lower bound directly, the entropy term $\cH(\bs{\cC_t})$ involves high-dimensional variables and is not easy to compute. 
Besides, it is also non-trivial to find an appropriate proposal distribution $q(\bs{C^t}|\bs{C^p})$. Therefore, we adopt a different approach for obtaining a novel lower bound on the mutual information quantity, as described above.

\section{Pseudo Code of Algorithms To Optimize LSH for Dialog Modeling}

In the following, we discuss the optimization of the reference set.
		
{ \bf Optimizing Reference Set. \\}
\begin{algorithm*}[th]
\caption{
% \small
\csizenine
Optimizing Reference Set in LSH-RkNN or LSH-RMM for Dialogue Modeling 
% by Maximizing Our MI LB
}
% \scriptsize
% \csize
% \small
\csizenine
\begin{algorithmic}[1]
\REQUIRE Training set $\bar{\bs{S}} = \{\bs{S}^p,\bs{S}^t\}$; initial and final size of reference set, $I$ and $M$ respectively; $\beta$ and $\gamma$ are the number of samples, as candidates for the reference set, and for computing the lower bound, respectively.
% \\
% \STATE $\bar{\bs{S}} = \{ S_1^p, \cdots, S_N^p, S_1^t, \cdots, S_N^t \}$
% \COMMENT{patient \& therapist responses in same set as candidates for the reference set}
% % 
% \\
% \STATE $\bs{S}^p = \{ S_1^p, \cdots, S_N^p \}$
% \COMMENT{patient responses}
% % 
% \\
% \STATE $\bs{S}^t = \{ S_1^t, \cdots, S_N^t \}$
% \COMMENT{therapist responses}
% 
\\
\STATE $\bs{r}^d$ $\gets$ randomSubset($2N$, $I$)
\COMMENT{random subset of indices, of size $I$, from $\{ 1, \cdots, 2N \}$ for initialization of reference set}
\\
\COMMENT{optimizing the reference set up to size $M$ greedily}
\FOR{$j=1 \to M$}
% 
% \\
% \COMMENT{Optimize $j^{th}$ element in the reference set}
% 
\IF{$j > I$}
\STATE $\bs{r}^d \gets \{ \bs{r}^d, randomSubset($2N$, 1) \}$
\COMMENT{adding one more element in the reference set, that is to be optimized}
\ENDIF
\STATE $\bs{r}^{ref}$ $\gets$ randomSubset($2N$, $\beta$)\COMMENT{subset of the structures as candidates for the reference set}
\STATE $\bs{r}^{lb}$ $\gets$ randomSubset($N$, $\gamma$)\COMMENT{subset of patient/therapist responses pairs for computing the MI lower bound}
\STATE $\bs{K}^p \gets$ computeKernel($\bs{S}^p(\bs{r}^{lb})$, $\bar{\bs{S}}(\bs{r}^{d})$)
\COMMENT{$\gamma \!\!\times\!\! j$ size}
\STATE $\bs{K}^t \gets$ computeKernel($\bs{S}^t(\bs{r}^{lb})$, $\bar{\bs{S}}(\bs{r}^{d})$)
\COMMENT{$\gamma \!\!\times\!\! j$ size}
\STATE $\bar{\bs{K}}^p \gets$ computeKernel($\bs{S}^p(\bs{r}^{lb})$, $\bar{\bs{S}}(\bs{r}^{ref})$)
\COMMENT{$\gamma \!\!\times\!\! \beta$ size}
\STATE $\bar{\bs{K}}^t \gets$ computeKernel($\bs{S}^t(\bs{r}^{lb})$, $\bar{\bs{S}}(\bs{r}^{ref})$)
\COMMENT{$\gamma \!\!\times\!\! \beta$ size}
% 
% \STATE $\bs{mi}_{lb}$ $\gets$ $\bs{0}$
% 
\STATE $\bs{mi}_{lb}$ $\gets$ computeMILowerBound($\bs{K}^p, \bs{K}^t, \bar{\bs{K}}^p, \bar{\bs{K}}^t$)
\COMMENT{compute the MI lower bound for all the candidates $\bar{\bs{S}}(\bs{r}^{ref})$, using the kernel matrices, via computation of hashcodes}
% 
% \FOR{$l=1 \to \beta$}
% 
% \STATE $\bs{C}^p \gets$ computeKernelHashcodes($\bs{K}^p$)
% 
% \STATE $\bs{C}^t \gets$ computeKernelHashcodes($\bs{K}^t$)
% 
% \STATE $\bs{mi}_{lb}(l)$ $\gets$ computeMILowerBound($\bs{S}(\bs{r}^{lb})$)
% 
% \ENDFOR
% 
\STATE $\bs{r}^{d}(j)$ $\gets$ maxMILBDataIndex($\bs{mi}_{lb}$, $\bs{r}^{ref}$)
\COMMENT{choose the index with maximum value of MI lower bound, from the set of candidate indices $\bs{r}^{ref}$}
\ENDFOR
\RETURN $\bar{\bs{S}}(\bs{r}^d)$
\end{algorithmic}
\label{alg:opt_ref}
\end{algorithm*}
For hashing models LSH-RkNN and LSH-RMM described in the main paper, we can optimize the reference set, $\bs{S}^R$, for dialog modeling as described in the following.
 
For the selection of elements in $\bs{S}^R$, we use a greedy algorithm maximizing the proposed mutual information lower bound~(in \thmref{thm:mi_lb}); see the pseudo code in \algoref{alg:opt_ref}. We initialize a reference set of small size $I \ll M$, by randomly selecting responses from the training set of patient/therapist responses, i.e. $\bar{\bs{S}} = \{ S_1^p, \cdots, S_N^p, S_1^t, \cdots, S_N^t \}$; though, as noted before, the superset $\bar{\bs{S}}$ for the random selection can be any set of sentences/paragraphs, not necessarily coming from a dataset of patient/therapist responses. First, each element in the initial reference set is optimized greedily, and then more elements are added one by one until the reference set size grows to $M$. When optimizing each element in the set, for computing the MI lower bound, we sample $\gamma$ number of response pairs from the training set of patient/therapist responses pairs, $\{ (S_i^p, S_i^t) \}_{i=1}^N$. For computational efficiency, we adopt the idea of sampling for the candidate set as well, in each greedy optimization step, by sampling a subset of candidates of size $\beta$ from the set $\bar{\bs{S}}$.

The computation cost in the optimization is dominated by the number convolution kernel similarities, i.e. $O(\gamma(M^2+M\beta))$. In practice, we can keep low values of $\gamma$ as well as $\beta$; in our experiments, we use $\beta=1000, \gamma=100$, and vary the value of $M$ from $30$ upto $300$. A similar procedure can be used to optimize kernel parameters.

{\bf Optimizing Neural Network Architecture. \\}
\begin{algorithm*}[tp!]
\caption{
% \small
\csizenine
Optimizing Neural Architecture in LSH-RLSTM for Dialog Modeling
% Neural-Hashing Model for Dialogue Modeling by Maximizing Our MI LB   - {\bf TODO Shorten the title}
}
\csizenine
\begin{algorithmic}[1]
\REQUIRE Training dataset $\{\bs{S}^p$, $\bs{S}^t\}$, with $N$ pairs; maximum number of layers in neural language models, $L$; the number of samples for computing the MI lower bound, $\gamma$; values for units in a layer, $\bs{u} =$ \{4, 8, 16, 32, 64, None\}. 
% \\
% \STATE $\bar{\bs{S}} = \{ S_1^p, \cdots, S_N^p, S_1^t, \cdots, S_N^t \}$
% \COMMENT{patient \& therapist responses in same set as the reference set}
% % 
% \\
% \STATE $\bs{S}^p = \{ S_1^p, \cdots, S_N^p \}$
% \COMMENT{patient responses}
% % 
% \\
% \STATE $\bs{S}^t = \{ S_1^t, \cdots, S_N^t \}$
% \COMMENT{therapist responses}
% 
% \STATE $\bs{r}^d$ $\gets$ randomSubset($2N$, $I$)
% \COMMENT{random subset of indices, of size $I$, from $\{ 1, \cdots, 2N \}$ for initialization of reference set}
% \\
% \STATE $NN \gets [10, None]$\COMMENT{initialization of neural network with 10 units in the first layer}
% 
% \STATE $NU \gets \{10, 20, 40, 80, None\}$\COMMENT{choices for number of units 
% in a layer
% }
\\
\COMMENT{optimizing up to $L$ layers greedily}
\FOR{$j=1 \to L$}
\STATE $\bs{r}^{lb}$ $\gets$ randomSubset($N$, $\gamma$)\COMMENT{subset of patient/therapist responses pairs for computing the MI LB to optimize $j_{th}$ layer}
% \\
% 
% 
\COMMENT{Number of units in $j_{th}$ layer, None not applicable for $1_{st}$ layer}
\FOR{$l \in \bs{u}$}
\STATE $\bs{n}(j) \gets l$\COMMENT{$l$ units in $j_{th}$ layer of neural network}
\STATE $\bs{C}^p \gets$ computeHashcodes($\bs{S}^p(\bs{r}^{lb}), \bs{n}$)
\STATE $\bs{C}^t \gets$ computeHashcodes($\bs{S}^t(\bs{r}^{lb}), \bs{n}$)
\STATE $\bs{mi}_{lb}(l)$ $\gets$ computeMILowerBound($\bs{C}^p, \bs{C}^t$)
% 
% \STATE $\bs{mi}_{lb}$ $\gets$ computeMILowerBound($\bs{K}^p, \bs{K}^t, \bar{\bs{K}}^p, \bar{\bs{K}}^t$)
% \COMMENT{compute the MI lower bound for all the candidates $\bar{\bs{S}}(\bs{r}^{ref})$, using the kernel matrices, via computation of hashcodes}
% 
\ENDFOR
\STATE $\bs{n}(j)$ $\gets$ maxMILBIndex($\bs{mi}_{lb}$, $\bs{u}$)
\COMMENT{choose the units with maximum value of MI LB}
\STATE \textbf{if} $\bs{n}(j)$ is None \textbf{then} break out of loop \textbf{end if}
\ENDFOR
\RETURN $\bs{n}$
\end{algorithmic}
\label{alg:opt_nn_layers}
\end{algorithm*}

For neural networks based LSH~(LSH-RLSTM), we can optimize the number of layers and the units in each layer, by maximizing the proposed MI LB; see pseudo code in \algoref{alg:opt_nn_layers}. 

\section{Experimental Details on LSH Models}
LSTM models for each hash function in \emph{LSH-RLSTM}  are  trained using Adam~\cite{kingma2014adam}, with the learning rate $1e-3$, amsgrad=True, and $l_1$, $l_2$ regularization coefficients set to   $1e-4$.  We initialize a word in a response and its POS tag with a random  vector of size 30; for a single time step processing with in LSTM, word vectors of 10 adjacent words, along with their POS tags, are appended into a vector of size 600; this is required to avoid vanishing gradients since patient responses can be of length up to 8,000 words in the training dataset. For the $H$ number of LSTM models as neural-hash functions, same neural architecture, i.e., same number of layers and units, are used in each model. When optimizing the architecture of the LSTM models with \algoref{alg:opt_nn_layers} by maximizing our proposed MI LB~(\emph{MI LB Optimal}), we add layers one by one greedily up to maximum possible 5 layers~($L=4, \gamma=1000$), and try out different possible numbers of normal units in each layer, i.e., 4, 8, 16, 32, 64. (We keep the number of units small, since $\alpha$ is small. Also, during the optimization, we use $H=30$). When optimizing the Reference set with \algoref{alg:opt_ref}, we keep $\beta=1000, \gamma=100, I=20$.

{\em Similarity metric}. In case of \emph{kernel-hashing}, we use subsequence kernels~\cite{mooney2005subsequence} for computing similarity between two responses (subsequences of length up to 16 are matched), while similarity between a pair of words is computed as cosine between their word vector representations.

\subsection{Subsequence Kernel}
Let $S_i$ and $S_j$ be two sequences of tokens~(words), the convolution kernel similarity between $S_i$ and $S_j$ is defined as below~\cite{mooney2005subsequence}.
            
\begin{align*}
\csizeten
K(S_i, S_j)
=
\sum_{e=1}^{16}
\sum_{\boldsymbol{i}, \boldsymbol{j}: |\boldsymbol{i}|=|\boldsymbol{j}|=e}
\prod_{k=1}^{|\boldsymbol{i}|}
k(S_i(\bs{i}_k), S_j(\bs{j}_k))
\lambda^{l(\boldsymbol{i})+l(\boldsymbol{j})}.
\end{align*}

Here, $k(S_i(\bs{i}_k), S_j(\bs{j}_k))$ is the similarity between the $k_{th}$ tokens in the subsequences $\boldsymbol{i}$ and $\boldsymbol{j}$, of equal length~(up to value 16); $l(.)$ is the actual length of a subsequence in the corresponding sequence, i.e., the difference between the end index and start index~(subsequences do not have to be contiguous); $\lambda \in (0, 1)$ is used to penalize the long subsequences. Dynamic programming is used for efficient computation of the subsequence kernel.
    
We use the following expression for computing the kernel similarity, $k(a,b)$, between two tokens $a$ and $b$ using their respective word vector representations~(real valued column vectors), $\bs{w}_a$ and $\bs{w}_b$.
            
\begin{align}
k(a, b)
=
cs
\left(
1-
\frac{(1-cs)}{(1-\zeta)}
\right)_{+};
\ \ \ 
cs = \frac{\bs{w}_a^T \bs{w}_b}{||\bs{w}_a||_2||\bs{w}_b||_2},
\end{align}

Herein, $cs$ is cosine similarity between the two word vectors, $\bs{w}_a$ and $\bs{w}_b$; $()_{+}$ represents the positive part function; $\zeta \in [-1,1]$ is a parameter for \emph{compact support} of the kernel function.

The parameters $\lambda, \zeta$ are optimized by maximizing the proposed MI LB criterion in our dialog model.

\section{Additional Experiment Details}

\begin{table*}[tp!]
\centering
\tabsize
\begin{tabular}{p{16.75cm}}
\toprule
\patient{I did lose three pounds, did you notice that?}
\\
\therapist{That's great, I did notice that.}
\\
\rmm{Yes, you did.}
% {\bf RMM:} Yes, you did.
\\
\rknn{To help you with your diet?}
\\
\rlstm{Okay what's the explanation?}
\\
{\bf LSTM:} I don't want to be a lot of a lot of a lot of a lot of a lot of a lot of a lot of a lot of a lot of a lot of a lot of a lot of a lot of a lot of a lot of a lot of a lot of a lot of a lot of a lot of a lot of a lot of a lot of a lot of a lot of a lot of a lot of a lot of a lot of a lot of a lot of the way
\\
{\bf HRED:} Yeah. you
\\
{\bf VHRED:} Uh-huh. you
\\
\toprule
\patient{Well, first of all, we've never been able to, when I first come to see you in July you highly recommended and I refused to go into this day treatment or some type of a hospital and I refused and you put me on medicine. And the medicine helped a great, great deal. I have been to 4 different psychiatrists and they've put me on Lithium and they've done other things and none of that stuff worked. And when I come to see you I was real skeptic but I was reaching out for help.}
\\
\therapist{Um-hum.}
\\
\rmm{I see.}
\\
\rknn{It does?}
\\
\rlstm{You mean its puzzling why? I suppose it's very depressing too.}
\\
{\bf LSTM:} I don't want to be a lot of a lot of a lot of a lot of a lot of a lot of a lot of a lot of a lot of a lot of a lot of a lot of a lot of a lot of a lot of a lot of a lot of a lot of a lot of a lot of a lot of a lot of a lot of a lot of a lot of a lot of a lot of a lot of a lot of a lot of a lot of the way
\\
{\bf HRED:} Okay. you
\\
{\bf VHRED:} Uh-huh.
\\
\toprule
\patient{Which is stupid because like, ya know, (sniffles) I guess if it's not what they like, then it's not what they like and they can like do something else, but like (sniffles) ya know there's some psychiatrists who charge like \$300 an hour. If you did that you would really have to work like...if you worked an hour a day five days a week that would be fifteen hundred dollars a week. Like...you wouldn't have to work at all...like barely. I mean, though, most psychiatrists probably don't charge \$300 an hour...yeah...it's just kinda ridiculous that...}
\\
\therapist{I'm sorry you're having such trouble getting...getting access to the care that you need (pause).}
\\
\rmm{You got to do.}
\\
\rknn{Oh yeah, you never tried Lithium?}
\\
\rlstm{And you ought not to just shove it away out of your life because you will need it again.}
\\
{\bf LSTM:} Uh-huh. you
\\
{\bf HRED:} Yeah. you
\\
{\bf VHRED:}  Uh-huh. you
\\
\toprule
\patient{I don't... I guess that's the problem right now. I guess that's what I'm grappling with. I guess that's what I'm amazed about. I think, you know, the hypothesis that you just presented about what I'm doing probing, you know, fucking you over, you know, all of these things (PAUSE) it's plausible to me. And that's freaky because my experience of it is just, you know, just being pinned to the wall.}
\\
\therapist{Right. So... (PAUSE) Maybe the (PAUSE) sort of... (PAUSE) If I think about the sort of world that that one part is living in, the sort of fucking me over part, I imagine it's a world where that goes both ways, where you can be coming here for months and months and trying and not getting anywhere with this. And, you know, getting up and doing your part and paying money sort of or, you know, you know what I mean. And, you know, and still get nothing. Which is how you felt at some moments recently.}
\\
\rmm{Could be.}
\\
\rknn{Because nobody's helping you.}
\\
\rlstm{The thing, the thing I'm trying to get a feel for is what happened that was good? What happened?}
\\
{\bf LSTM:} Okay, you
\\
{\bf HRED:} M-hmm. you
\\
{\bf VHRED:} Okay, you
\\
\toprule
\patient{Yeah. I mean, it'll start, yknow, like right now, I mean, you're familiar with the weather patterns and things like that. It's not getting, I mean, the light is going to start to diminish, but the cold and having to be stuck in the house and everything all day isn't going to start for another month. Yknow, I'm still fine right now. Um, would you want me to call you then when I was going to start to take the 200 to let you know the beginning of it?}
\\
\therapist{Yeah, of course. Of course, you could do that.}
\\
\rmm{Yeah you probably could.}
\\
\rknn{So you get a little.}
\\
\rlstm{Right? And so just something to think about. It doesn't mean that it has to happen that way, but it can. And so the times where I may think that applies, I may bring it up. Because it's about relating your past relationships to your present relationships. And even how you relate in here with me. And so we may talk about that at some point.}
\\
{\bf LSTM:} I don't want to be a lot of a lot of a lot of a lot of a lot of a lot of a lot of a lot of a lot of a lot of a lot of a lot of a lot of a lot of a lot of a lot of a lot of a lot of a lot of a lot of a lot of a lot of a lot of a lot of a lot of a lot of a lot of a lot of a lot of a lot of a lot of a lot
\\
{\bf HRED:} Yeah. you
\\
{\bf VHRED:} Okay. you
\\
\toprule
\patient{The fact that I wanted to do things that he didn't and then he felt guilty and I was like, \"Well, I mean it's not your fault because you're depressed and disappointed, too, and couldn't not be disappointed and stuff, too. Instead just focus on cuddling.}
\\
\therapist{That's not satisfying for you.}
\\
\rmm{Such as?}
\\
\rknn{Yeah.}
\\
\rlstm{One more thing, you just don't look at them enough.}
\\
{\bf LSTM:} Uh-huh. you
\\
{\bf HRED:} M-hmm. you
\\
{\bf VHRED:} Uh-huh. you
\\
\toprule
\patient{ Well I guess because there's truth to it when you go (ph), \"Okay, well what are you avoiding?\" in essence. I mean, there's truth to that. Because I ... because working in here, I agree, that's a thing I want to do is be focused on how I'm feeling. This whole thing with my family not being able to show feelings. By the way, I just have to drive over this scenic outlook and tell you that I, you know, I did talk to my mother about ...}
\\
\therapist{Now why are you doing that now?}
\\
\rmm{It's up to you.}
\\
\rknn{Yeah, people get really provocative.}
\\
\rlstm{How so?}
\\
{\bf LSTM:} I don't want to be a lot of a lot of a lot of a lot of a lot of a lot of a lot of a lot of a lot of a lot of a lot of a lot of a lot of a lot of a lot of a lot of a lot of a lot of a lot of a lot of a lot of a lot of a lot of a lot of a lot of a lot of a lot of a lot of a lot of a lot of a lot of the way
\\
{\bf HRED:} M-hmm. you
\\
{\bf VHRED:} Uh-huh. you
\\
\toprule
\patient{I hope so, I don't know what the heck that is, I don't' have any idea what that is, oh well, okay.}
\\
\therapist{Okay.}
\\
\rmm{And doing something that feels more like you.}
\\
\rknn{And you felt like that was - somehow you just couldn't do it I think.}
\\
\rlstm{You thought about that.}
\\
{\bf LSTM:} is a lot of a lot of a lot of a lot of a lot of a lot of a lot of a lot of a lot of a lot of a lot of a lot of a lot of a lot of a lot of a lot of a lot of a lot of a lot of a lot of a lot of a lot of a lot of a lot of a lot of a lot of a lot of a lot of a lot of a lot of a lot of a lot of a lot of
\\
{\bf HRED:} Okay. you
\\
{\bf VHRED:} Okay, you
\\
\toprule
\end{tabular}
\caption{
Textual responses generated by different systems for Depression Therapy dataset, along with ground truth patient and therapist responses.
}
\label{tab:gen_responses}
\end{table*}

\begin{table*}[tp!]
\centering
\csize
\begin{tabular}{p{16.75cm}}
\toprule
Yeah, here's hoping.\\
It's going to keep on being a struggle.\\
There isn't any, really anyone (ph) inside?\\
The Petition is the part that—\\
No, I don't. I really don't except that partly it's a fear of being further condemned by her. I mean, she condemns me for everything I am and everything I do.\\
So that there was again the concern with the - with [NAME].\\
Yeah. And so we didn't talk all the way home at all. And as we didn't talk, I think we were both growing angry. And so then we sat and we did talk for a long time. And that was good. Well, it was good. It was more...we talked more deeply about ourselves and our feelings than we were in the past without being angry at each other.\\
Yeah.\\
You've got your mother and sister.\\
Maybe if things are still horrible. I am hoping by next week they will be\\
When I told you that, did you remember what you felt?\\
And how to use that too.\\
You know people nearby pretty much though is you know? Also I think it's also he cannot ... he's been already like conditioned into, if he gets angry or has any ill feelings towards certain members of the family that's going to be it. Because he is no longer going be, you know ...\\
Well, that's what we're going to talk about.\\
From where?\\
I mean, you've been, I think it's great, you going every week to see [NAME OTHER], just about?\\
What's that, hon?\\
Yes.\\
Well yeah, like they didn't want their kids to be the real dummies in the neighborhood (laughter). But it's not - my father, it's not that he likes to brag on his kids if their not there. I mean he'd never say anything nice about us in front of us. But I guess it's the teachers that really bother me. I mean why get a kid an answer book. I can't - I mean, of course, I could have not cheated, but i And everything else I've done was very easy. My clarinet lessons; [I had beef cattle] (ph); I was in girl scouts. And, I mean, all I had to do was pick them out. I never had do any work. The boys always did the work, and then I went to the fair and got the purple ribbons.\\
Was it like defense-type stuff?\\
When you think of that moment in the car, how true do the words, "I can go on and thrive" feel on a 1-7 scale, with 1 being completely false and 7 being completely true?\\
I'm not seeing anybody right now.  I've got to, I've got to worry about me first.\\
I don't know. I thought of that all the time. Like how I've seen have big boxes of Kleenex usually expect the girls to cry.\\
It's easier with the groups you so about.\\
And same at your church I think.\\
Yeah.\\
Okay.\\
And with that sort of a person.  But because he is your biological father, there's a certain obligation and you are kind enough to do what has to be done.  That for you to have feelings wouldn't make much sense to me.  Of course, where, where are the feelings to come from?  The feelings would come from the acts of kindness and caring, compassion.  If they were not there, what should you feel?  But you are, nevertheless, kind enough to do the decent thing.  So, so that's one thing.  But how do you feel about that?  What I've just said?\\
I want a safe place out there.\\
No.  I had it during finals my first year of grad school and during my second year probably for like four months towards the end.\\
Yeah. I get that.\\
Okay, that's okay.\\
Once they send you the check -\\
It all seems so bad to you, it's a disillusion.\\
Yeah.\\
I said you don't want what I'm thinking on your tape.\\
So after I took one half at night, I was able to get up in the morning.\\
If I had asked you beforehand what they were going to do...?\\
You drink because you're lonely.\\
That's all right.\\
Yeah, in other words maybe I shouldn't have gotten so upset. Whereas it wasn't the most pleasant thing I should do. And like he was trying to say, you know, can't you just stay here tonight and leave tomorrow for college, see your girlfriend. And I've forgotten, it wasn't until like I just got the mail just before I came here and I was really, I didn't want to open it. It was just two Valentine's. It didn't say anything, you know, except love, Daddy and [NAME] and love, [NAME], but...\\
You went out\\
Um-hum.\\
Let's just pretend for a moment. Let's pretend that I'm your boss.\\
Okay. How old are you now?\\
Right. Well, a lot of it was like, before Christmas I was really, really snowed under with stuff and I had to work every day and I had to work late almost every day, and somehow even just the hour coming here was really a lot. Plus, I was really functioning on, 'let me just get through with work' because I had so many hours that I had to get through by Christmas or I couldn't go home for Christmas, and it was sort of, 'let me just get through that and think about things later'.\\
I was starting, you know, itching, it's almost for a month, a month and a half, I keep itching a lot over here in my face.\\
I feel like I've lost credentials and hope over...\\
Will you try out something again right now what you would find to be a response to Shelley given the fact of last week for example?\\
The rapport was good enough for that.\\

\toprule
\end{tabular}
% \vspace{-3mm}
\caption{
% \csize
We show first 50 responses~(in raw text format) that are selected greedily for the reference set~($\bs{S}^R$) in \emph{LSH-RkNN} model, out of 76,000 responses from the train set, with \algoref{alg:opt_ref}.}
\label{tab:reference_responses}
% \vspace{-1.5mm}
\end{table*}

% \input{dialogueGenerated.tex}

% \input{refSetRMM.tex}

% \newpage

% \section{Sections to be added later for the final paper submission}
% \subsection{Semisupervised Learning}

% \subsection{Optimizing Kernel Parameters}
	
% \subsection{Faster computation Strategies}
% \paragraph{Lazy greedy evaluation}
% \paragraph{Stochastic estimate of the lower bounds}
% \paragraph{Parallel computing}

% \subsection{Discussion on Hashing Algorithm}
% Discussion subtle details like conditions for correlation between hashcode bits, and how we are optimizing attention in text with learning of the reference set

% \subsection{Textual Response Inference from Hashcode}
% Having learned the hashing model, a set of unlabeled sentences, as potential responses from automated therapists, can be hashed. If the number of hashcode bits is very large, sublinear time algorithms can be used for efficient similarity search (nearest neighbors) in hamming spaces~\cite{norouzi2014fast,komorowski2017random}.
	
% We need to choose one of these algorithms.
